# Supplementary material for: DeRS: Towards Extremely Efficient Upcycled Mixture-of-Experts Models
Source: arXiv:2503.01359 source file (2025-03-03)
Supplement: Supplementary file 1 [file _supplementary.tex]

% \input{_constants}
% \review % \review OR \cameraready

% \documentclass[10pt,twocolumn,letterpaper]{article}
% \input{cvpr_header}
% \myexternaldocument{_main}
% \begin{document}

% %% TITLE
% \title{\paperTitle}
% \author{\authorBlock}
% \maketitlesupplementary
% %%

% \appendix
% \input{sec/X_appendix}

% \end{document}
