# Supplementary material for: DeRS: Towards Extremely Efficient Upcycled Mixture-of-Experts Models
Source: arXiv:2503.01359 source file (2025-03-03)
Supplement: Supplementary file 2 [file ablation_DeRS_SM.tex]

\begin{table}[!t]
\caption{\textbf{}}
  \label{tab:ablation_DeRS_SM}
  \resizebox{1.0\linewidth}{!}{
  
  \centering
  \begin{tabular}{c|c|cc|c}
    \toprule
     \textbf{\begin{tabular}[c]{@{}c@{}}DeRS-SM\\ Ratio\end{tabular}} & \textbf{\begin{tabular}[c]{@{}c@{}}Added\\ Params.\end{tabular}} & \textbf{HumanEval (+)} & \textbf{MBPP (+)} & \textbf{Overall} \\
    \midrule
    0.9999 & \textcolor{gray}{0.81B}+0.72M & 62.8 (60.4) & 63.7 (51.6) & 59.6 \\
    0.999  & \textcolor{gray}{0.81B}+3.64M & 64.0 (60.4) & 63.4 (51.6) & 59.9 \\ 
    0.99   & \textcolor{gray}{0.81B}+32.9M & 64.6 (61.6) & 62.7 (51.4) & 60.1 \\ 
    0.9    & \textcolor{gray}{0.81B}+325M & 66.5 (62.8) & 63.4 (51.4) & 61.0 \\ 
    \bottomrule
  \end{tabular}}
\end{table}
